# Supplementary material for: Gravitational Lenses in UNIONS and Euclid (GLUE) I: A Search for Strong Gravitational Lenses in UNIONS with Subaru, CFHT, and Pan-STARRS Data
Source: arXiv:2505.05032 source file (2026-06-08)
Supplement: Supplementary file 1 [file appendix.tex]

\begin{minipage}{\textwidth}
    \centering
    \hspace{-1.25cm}
    \includegraphics[width=0.85\textwidth]{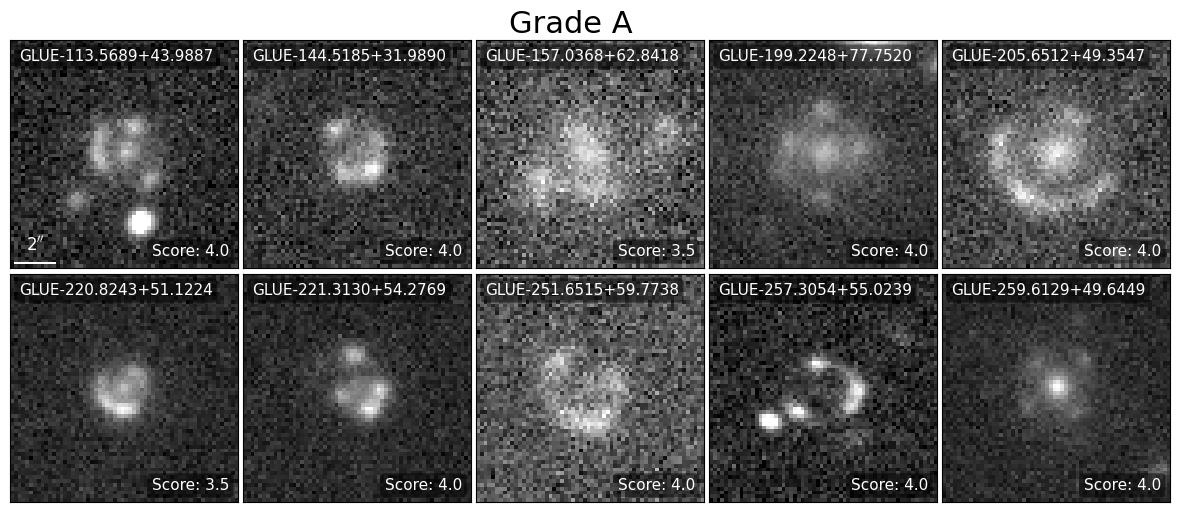} % Adjust width as needed
    % \captionof{figure}{Caption for image 1}
    \vspace{1em} % Space between images
    \hspace{-1.25cm}
    \vspace{-0.4cm}
    \includegraphics[width=0.85\textwidth]{figures/UNIONS_cands_Bs_zoom_g.png} % Adjust width as needed
    % \captionof{figure}{Caption for image 2}
    \vspace{1em} % Space between images
    \hspace{-1.25cm}
    \vspace{-0.5cm}
    \includegraphics[width=0.85\textwidth]{figures/UNIONS_cands_Cs_zoom_g.png} % Adjust width as needed
    \captionof{figure}{\footnotesize }
\end{minipage}
